# Supplementary material for: Approximation algorithms for the MAXSPACE advertisement problem
Source: arXiv:2006.13430 source file (2023-05-08)
Supplement: Supplementary file 1 [file appendix.tex]

% !TeX spellcheck = en_US

\begin{proof}[of Lemma~\ref{lemma:1}]
  The loops of Lines~\ref{linha:1} and~\ref{linha:42} execute a constant number of iterations, since~${|\calt| = 2^K}$ and the number of subsets of~$\calt$ is~$2^{2^K}$. The inner loop (Line~\ref{linha:5}) executes a polynomial number of iterations since~$|\PW|$ is polynomial. Then, the algorithm executes in polynomial time.
\end{proof}

\begin{proof}[of Lemma~\ref{lemma:3}]
  The maximum flow is solved in polynomial time in the size of graph~$H$~\cite{ahuja2017network} and~$H$ is polynomial in the size of the instance since it has exactly one vertex per small ad and a constant number of vertices for types. The~$\Call{Rouding}{}$ algorithm is also polynomial, by Lemma~\ref{lemma:1}. Then, Algorithm~\ref{alg:2k} is polynomial in the instance size.
\end{proof}

%\todo{onde tiver falando de pattern, mudar para configuration}
\begin{proof}[of Lemma~\ref{lemma:6}]
  The number of configurations for large ads is polynomial, by Lemma~\ref{lemma:large}. Thus, the loop of Line~\ref{linha:4} executes a polynomial number of iterations. Also, the number of capacity vectors which are compatible with each such configuration is at most a constant, by equation~\eqref{eq:4}. Thus, the loop of Line~\ref{linha:6} executes a polynomial number of iterations. The call to~\Call{AlgP$_\varepsilon$}{} also runs in polynomial time, by Lemma~\ref{lemma:3}. Therefore, the algorithm runs in polynomial time.
\end{proof}
